# Supplementary material for: Efficient Computation of High-Dimensional Penalized Generalized Linear Mixed Models by Latent Factor Modeling of the Random Effects
Source: arXiv:2305.08201 source file (2024-04-16)
Supplement: Supplementary file 1 [file Heiling_et_al_Supporting_Information_Effficient_computation_of_high_dimensional_penalized_generalized_linear_mixed_models_by_latent_factor_modeling_of_the_random_effects.pdf]

**Supporting Information for ‘Efficient Computation of High-Dimensional  
Penalized Generalized Linear Mixed Models by Latent Factor Modeling of the  
Random Effects’**

**Hillary M. Heiling<sup>1,\*</sup>, Naim U. Rashid<sup>1</sup>, Quefeng Li<sup>1</sup>, Xianlu L. Peng<sup>2</sup>, Jen Jen Yeh<sup>2,3,4</sup>,  
and Joseph G. Ibrahim<sup>1</sup>**

<sup>1</sup>Department of Biostatistics, University of North Carolina Chapel Hill, Chapel Hill, NC

<sup>2</sup>Lineberger Comprehensive Cancer Center, University of North Carolina at Chapel Hill, Chapel Hill, NC

<sup>3</sup>Department of Surgery, University of North Carolina Chapel Hill, Chapel Hill, NC

<sup>4</sup>Department of Pharmacology, University of North Carolina Chapel Hill, Chapel Hill, NC

\**email*: hheiling@live.unc.edu

This paper has been submitted for consideration for publication in *Biometrics*

## 1. Web Appendix: Supplementary Simulation and Case Study Materials

### 1.1 Model Selection

This section provides details on how the **glmmPen\_FA** algorithm selects the optimal tuning parameter combination. In all simulations and analyses discussed in this paper, we set the random effects equal to the fixed effects (i.e.  $p = q$ ) and let the algorithm select the fixed and random effects.

The algorithm runs a computationally efficient two-stage approach to pick the optimal set of tuning parameters. In the first stage of this approach, the algorithm fits a sequence of models where the fixed effect penalty is kept constant at the minimum value of the fixed effects penalty sequence, labeled here as  $\lambda_{0,min}$ , and the random effects penalty proceeds from the minimum random effect penalty, labeled  $\lambda_{1,min}$ , to the maximum value  $\lambda_{1,max}$ . The best model from this first stage is then identified using the BIC-ICQ criterion (Ibrahim et al., 2011). This first stage identifies the optimal random effect penalty value,  $\lambda_{1,opt}$ . In the second stage, the algorithm fits a sequence of models where the random effects penalty is kept fixed at  $\lambda_{1,opt}$  and the fixed effects penalty proceeds from its minimum value  $\lambda_{0,min}$  to its maximum value  $\lambda_{0,max}$ . The overall best model is chosen from the models in the second stage.

We have found this two-stage model selection approach to work very well in practice (see Section 3 for performance results).

### 1.2 Tuning parameter selection

The default maximum penalty, labeled here as  $\lambda_{max}$ , was calculated as the penalty that would penalize all of the fixed effects to 0 when no random effects are in the model. We used code from the **ncvreg** R package (Breheny and Huang, 2011) to calculate this value.

For all Binomial outcome variable selection simulations and case study analyses where the total number of predictors was 100 or less, we used the following sequence of penalties for both

the fixed effects and the rows of the  $\mathbf{B}$  matrix: a sequence of 10 penalties from  $0.05\lambda_{max}$  to  $\lambda_{max}$ , with penalty values equidistant from each other on the log scale.

For all Binomial outcome variable selection simulations and case study analyses where the total number of predictors was 500, we used the following sequence of penalties: a sequence of 10 penalties from  $0.15\lambda_{max}$  to  $\lambda_{max}$  for the fixed effects, and a sequence of 10 penalties from  $0.10\lambda_{max}$  to  $\lambda_{max}$  for the rows of the  $\mathbf{B}$  matrix, with penalty values equidistant from each other on the log scale. In simulations not shown here, using a consistent sequence of 10 penalties from  $0.10\lambda_{max}$  to  $\lambda_{max}$  for both sets of parameters resulted in very similar final results, but accomplished in more time; using a consistent sequence of 10 penalties from  $0.15\lambda_{max}$  to  $\lambda_{max}$  for both sets of parameters decreased the random effect true positive results.

For the Poisson outcome variable selection simulations, a penalty sequence with larger values was needed for both the fixed effects and rows of the  $\mathbf{B}$  matrix due to the nature of how the data was simulated and fit. In these simulations, the covariate values  $x_{ki,j}$  were simulated from a  $N(0, \sigma = 0.10)$  distribution for  $j = 1, \dots, p$  and left unstandardized in the algorithm, whereas in the binomial simulations, the covariate values were simulated from the standard normal distribution  $N(0, 1)$  and then standardized so that  $\sum_{k=1}^K \sum_{i \in n_k} x_{ki,j} = 0$  and  $\mathbf{x}_j^T \mathbf{x}_j / N = 1$  for each  $j$ . The fixed effects penalty sequence included  $0.30\lambda_{max}$  and  $(\delta_{0,1}, \dots, \delta_{0,12}) * \lambda_{max}$ , where  $\delta_{0,i} = 2 + (i - 1)$ . The random effect penalty sequence applied to rows of the  $\mathbf{B}$  matrix included  $0.30\lambda_{max}$  and  $(\delta_{1,1}, \dots, \delta_{1,11}) * \lambda_{max}$ , where  $\delta_{1,i} = 0.5 + (i - 1)$ .

### 1.3 Initialization and Convergence - *glmmPen-FA*

The fixed effects  $\boldsymbol{\beta}^{(0)}$  and random effects covariance terms  $\mathbf{b}^{(0)}$  are initialized at iteration  $s = 0$  in one of two ways. We discuss first the initialization procedure used when the package **glmmPen** is used to fit a single model or the first model in the sequence of models fit for variable selection. In this scenario, the fixed effects  $\boldsymbol{\beta}^{(0)}$  are initialized by fitting a ‘naive’ model

using the coordinate descent techniques of Breheny and Huang (2011) assuming no random effects.

Based on the initialized fixed effects  $\beta^{(0)}$ , the predictors with non-zero initialized fixed effects are also initialized to have non-zero random effects (i.e. the corresponding rows of the  $\mathbf{B}$  matrix are set to non-zero values), and predictors with zero-valued initialized fixed effects are initialized to have zero-valued random effects (i.e. the corresponding rows of the  $\mathbf{B}$  matrix are set to zero). By default, the starting  $\mathbf{B}$  matrix elements are initialized as  $\sqrt{0.10/r}$ , where  $r$  is the estimated number of latent factors. The corresponding initialized covariance matrix  $\Sigma = \mathbf{B}\mathbf{B}^T$  will have all non-zero elements equal to 0.10.

The E-step MCMC chain of the sample of the posterior density  $\phi(\alpha_k | \mathbf{d}_{k,o}; \theta^{(s)})$  for groups  $k = \{1, \dots, K\}$  is initialized in iteration  $s = 1$  with random draws from the standard normal distribution. For all following iterations  $s > 1$ , the MCMC chain is initialized with the last draw from the previous iteration  $s - 1$ . At iteration  $s = 0$ , we sample  $M = 100$  posterior samples from each group, and  $M$  increases to a max of 500 as the iteration number  $s$  increases.

When the algorithm performs variable selection, we initialize models with previous model results. After the first model is fit in the variable selection procedure, the fixed effects, random effects covariance matrix, and random effects MCMC chain are initialized using results from a previous model fit.

The EM algorithm is considered to have converged when the following condition is met at least 2 consecutive times (default) or until the maximum number of EM iterations (25) is reached:

$$\|(\beta^{(s)T}, \mathbf{b}^{(s)T})^T - (\beta^{(s-t)T}, \mathbf{b}^{(s-t)T})^T\|_2^2 / d_n^{s-t} < \epsilon_{EM} \quad (1)$$

where the superscript  $(s - t)$  indicates  $t$  EM iterations back (default  $t = 2$ ),  $\|\cdot\|_2^2$  represents the  $L_2$  norm, and  $d_n^{s-t}$  equals the total number of non-zero  $(\beta^T, \mathbf{b}^T)^T$  coefficients in iteration  $(s - t)$ . In other words, the algorithm computes the average Euclidean distance between the

current coefficient vector  $(\boldsymbol{\beta}^T, \mathbf{b}^T)^T$  and the coefficient vector from  $t$  EM iterations back and compares it with  $\epsilon_{EM} = 0.0015$ .

The M-step algorithm is considered to have converged when the following condition is met or until the maximum number of iterations (50) is reached:

$$\max_j |\beta_j^{(s,f+1)} - \beta_j^{(s,f)}| \cap \max_{t,h} |b_{th}^{(s,f+1)} - b_{th}^{(s,f)}| < \epsilon_m, \quad (2)$$

where  $b_{th}$  is an individual element of  $\mathbf{b}_t$ , which is the  $t$ -th row of the  $\mathbf{B}$ . The value of  $\epsilon_m$  was set to 0.001.

#### 1.4 Initialization and Convergence - *glmmPen*

The initialization and convergence of *glmmPen* in these simulations and analyses were very similar to the initialization and convergence of *glmmPen\_FA* with the exception of the initialization of the random effect covariance matrix. This starting variance is initialized in an automated fashion. First, a GLMM composed of only a fixed and random intercept is fit using the **lme4** package. The random intercept variance from this model is then multiplied by 2, and this value is set as the starting values of the diagonal of the random effects covariance matrix. Similar to the **glmmPen\_FA** random effect initialization, the predictors are initialized to have non-zero random effects if they are also initialized to have nonzero fixed effects; otherwise, predictors are initialized to have no random effects.

#### 1.5 Elastic Net Penalty

We extended our simulations on variable selection in Binomial data by adding correlations between the simulated covariates and adjusting for this correlation using the Elastic Net penalization approach. Elastic Net penalization balances the MCP, SCAD, or LASSO penalties with ridge regression. This balance between ridge regression and the other penalty is dictated by a value we label as  $\pi$ , where  $\pi = 1.0$  represents the MCP penalty and  $\pi = 0$  represents ridge regression.

In these simulations, we set the sample size to  $N = 2500$  and number of groups to  $K = 25$ , with an equal number of subjects per group. There were  $p = 100$  total predictors and 10 true predictors with non-zero fixed and random effects. We considered four types of correlations between the predictors. In three of the four correlation types, the correlation between all covariates was set to a common value of 0.2, 0.4, or 0.6, and the variance of the covariates was set to 1. In the fourth correlation type, we randomly selected 100 of the 110 covariates used in the case study (see Web Appendix Section 1.6 for details) and calculated the Spearman correlation of these 100 covariates. In all four correlation cases, we simulated the covariates from a multivariate normal distribution with mean 0 and covariance matrix set to the correlation matrices described above.

We simulated the random effects covariance matrix using  $r = 3$  and the corresponding moderate  $\mathbf{B}$  matrix described in the main manuscript. The 10 true fixed effects  $\beta$  coefficients were set to 1. The generation of the binary responses from a logistic mixed effects model proceeded as described in Section 3.1.

We performed variable selection on these simulated data using Elastic Net  $\alpha$  values of 0.1, 0.3, 0.5, 0.8, and 1.0, and we estimated the number of common factors  $r$  using the default Growth Ratio procedure described in Section 2.4.

A summary of the variable selection results—true positive percentages, false positive percentages, median time in hours to complete the procedure, and average absolute deviation for the fixed effects coefficients—is given in Web Appendix Table 1. A summary of the performance of the Growth Ratio estimation procedure is given in Web Appendix Table 2.

[Table 1 about here.]

[Table 2 about here.]

In general, increasing the correlation among the predictors decreases the average true positive

percentage. Within a particular correlation set-up, decreasing the value of the Elastic Net  $\pi$  tends to increase both the true positives and the false positives.

The Growth Ratio procedure tends to underestimate the number of common factors  $r$  as the correlation between the covariates increases. However, when the correlation between the covariates is high at a value of 0.6 and there is no adjustment for ridge regression (i.e.  $\pi = 1.0$ , equivalent to the MCP penalty), there are more instances of the Growth Ratio procedure overestimating  $r$ .

For low values of  $\pi$  and/or high correlation, some simulation replicates had model fit issues. Specifically, in certain situations, the random effect variances diverged to excessively large values. As a result, the BIC-ICQ model selection criteria could not be calculated for the model, and the model selection procedure was suspended. When  $\pi = 0.1$  and the correlation among the predictors was 0.4 or 0.6, this phenomena happened 25% or 26% of the time, respectively. When  $\pi = 0.1$  and the correlation was 0.2, this happened 2% of the time; when  $\pi = 0.3$  and the correlation was 0.4 or 0.6, this happened 1% or 3% of the time, respectively; when  $\pi = 1.0$  and the correlation was 0.6, this happened 1% of the time. The simulations summarized in Web Appendix Table 1 do not include results from these problematic simulation replicates.

### 1.6 Case Study: Study Information and Data Processing

In this section, we provide more information about the individual studies contained within the dataset and describe how we set up the data for the case study analyses in Section 4. More complete coding details are provided in the GitHub repository [https://github.com/hheiling/paper\\_glmmPen\\_FA](https://github.com/hheiling/paper_glmmPen_FA).

The studies used in these analyses are summarized in Web Appendix Table 3, which contains the gene expression platform information (all RNA-seq), the sample sizes, and the percent of the samples that were classified into the basal subgroup.

[Table 3 about here.]

Web Appendix Table 3 provides the dataset abbreviations, their respective citations, their sample sizes, and the percent of the subjects within each study that were classified into the basal subtype. The sample sizes listed in the table—and used in the analyses—were smaller than the studies’ total sample size as we removed subjects with missing tumor grade information, normal tissue samples, and those who did not have primary tumor samples of sufficient quality. All five datasets had RNA-seq data for 60,230 total gene symbols for each subject. Of those, 432 were also part of the 500 member gene list that Moffitt et al. (2015) specified as relevant for classifying subjects into the basal vs classical subtypes (this gene list is also provided within the aforementioned GitHub repository).

There were some significant correlations between some of these 432 genes, as evaluated by Spearman correlations. In order to avoid having very highly correlated covariates in the analyses, we decided to combine highly correlated genes together into meta-genes. We accomplished this by applying a hierarchical clustering algorithm to the the genes using the `pheatmap::pheatmap()` R function (Kolde, 2019) to the absolute values of the Spearman correlation matrix. We then cut the tree using the `stats::cutree()` R function (R Core Team, 2021) at a height of 2. This produced a total of 119 clusters. For clusters that represented two or more genes, we added the raw RNA-seq gene expression of all participating genes to get the new cluster covariate values. We further removed 9 of the 119 of these clusters so that all pairwise Spearman correlations were below 0.9. The remaining 110 clusters were rank-transformed on the subject level, and these rank-transformed covariates were used in the case study analyses.

The cancer subtype outcome—basal or classical—was calculated using the clustering algorithm specified in Moffitt et al. (2015). For each study individually, this clustering algorithm was applied to the RNA-seq gene expression for the 432 genes described above, where the

distance matrix was the Euclidean distance and the assumed number of clusters was set to two.

### 1.7 Case Study: Sensitivity Analyses

We performed sensitivity analyses on our case study by running the Elastic Net variable selection procedure with alternative values of  $\pi$ —the value that represents the balance between ridge regression and the MCP penalty ( $\pi = 0$  represents ridge regression,  $\pi = 1$  represents the MCP penalty)—and alternative values for the number of latent common factors  $r$  (for the **glmmPen\_FA** procedure). Based on the results in Web Appendix Table 1,  $\pi$  values between 0.5 and 1.0 were likely to have good selection results for the correlation structure of the covariates in the dataset. We fit the variable selection procedure using  $\pi = \{0.6, 0.7, 0.8, 0.9, 1.0\}$ . The **glmmPen** procedure assumed an independent random effects covariance matrix.

We first discuss the **glmmPen\_FA** sensitivity results. In addition to estimating the number of latent common factors using the Growth Ratio procedure, which estimated a value of  $r = 2$ , we also fit the model assuming  $r = 3$  because the simulations given in Web Appendix Section 1.5 indicated that the Growth Ratio method may underestimate  $r$ . Regardless of whether  $r$  was estimated as 2 using the Growth Ratio procedure or set to 3 manually, the coefficient values and selection results were very consistent for each value of  $\pi$ . The single exception was when the  $\pi = 0.9$  selection procedure included another cluster covariate in the best model for  $r = 3$  but not  $r = 2$ ; even in this case, the fixed effect coefficient for the additional covariate was relatively small.

In terms of fixed effects, the values  $\pi$  between 0.6 and 1.0 gave very consistent results within the **glmmPen\_FA** procedure. The 8 covariate clusters described in the main paper Table 6 were consistently chosen across the different values of  $\pi$ , with the exception of cluster 45, which was excluded from the best model when  $\pi = \{0.6, 0.8\}$ . A 9-th cluster, cluster 75 (genes SERPINB3 and SERPINB4) was included when  $\pi = 0.9$  and  $r$  was set to 3; the fixed effect

coefficient for this covariate was relatively small in comparison with the other fixed effect coefficients.

For random effects, values of  $\pi \leq 0.8$  consistently selected 0 random effect slopes (random intercept only for random effects) within the **glmmPen\_FA** procedure. For  $\pi = \{0.9, 1.0\}$ , clusters 25, 58, and 91 had non-zero random effects. However, when  $\pi = 1.0$ , the variances of these random effects became suspiciously large (variance values approximately between 9 and 30), indicating a poor model fit for  $\pi = 1.0$ . The variances of these same random effects when  $\pi = 0.9$  were instead approximately between 1 and 2.

We chose to report the **glmmPen\_FA** results of  $\pi = 0.7$  in the main manuscript for several reasons. Based on the fact that we had a range of correlations among the covariates in the dataset, including some pairwise correlations greater than 0.6, we felt it was appropriate to fit the variable selection procedure with  $\pi < 1.0$ ; furthermore, based on the best model results, the  $\pi = 1.0$  showed poor model fit results for the random effects. When choosing between the other values of  $\pi$ , the  $\pi = 0.7$  results contained the consistently selected 8 cluster covariates, and these results did not contain any random slopes, which was also consistent across most of the values of  $\pi = \{0.6, 0.7, 0.8, 0.9\}$ .

The times to complete the **glmmPen\_FA** variable selection procedure was between 0.4 and 1.0 hours for  $\pi = \{0.6, 0.7, 0.8, 0.9\}$  (this range includes  $r$  either 2 or 3). When  $\pi = 1.0$ , the time to complete the procedure was 1.3 and 2.1 hours for  $r$  equal to 2 or 3, respectively.

The **glmmPen** procedure also consistently selected the 8 covariate clusters described in the main paper Table 6 to have non-zero fixed effects with the the following exceptions: procedure that used  $\pi = 0.7$  penalized out clusters 25 and 45, and the procedure that used  $\pi = 1.0$  penalized out cluster 75. With the exception of  $\pi = 0.6$ , **glmmPen** consistently selected clusters 25 and 58 to have non-zero random effects. The values of these slopes changed

depending on the value of  $\pi$ : variances of approximately 0.5 when  $\pi = \{0.7, 0.8\}$ , and variances greater than 1.0 when  $\pi = 0.9$ , and divergent values greater than 9 when  $\pi = 1.0$ .

The times in hours to complete the **glmmPen** variable selection procedure was 32.4, 37.8, 37.7, 51.2, and 68.2 for  $\pi$  equal to 0.6, 0.7, 0.8, 0.9, and 1.0, respectively.

## References

- Aguirre, A. J., Nowak, J. A., Camarda, N. D., Moffitt, R. A., Ghazani, A. A., Hazar-Rethinam, M., Raghavan, S., Kim, J., Brais, L. K., Ragon, D., et al. (2018). Real-time genomic characterization of advanced pancreatic cancer to enable precision medicine. *Cancer discovery* **8**, 1096–1111.
- Breheny, P. and Huang, J. (2011). Coordinate descent algorithms for nonconvex penalized regression, with applications to biological feature selection. *Annals of Applied Statistics* **5**, 232–253.
- Cao, L., Huang, C., Zhou, D. C., Hu, Y., Lih, T. M., Savage, S. R., Krug, K., Clark, D. J., Schnaubelt, M., Chen, L., et al. (2021). Proteogenomic characterization of pancreatic ductal adenocarcinoma. *Cell* **184**, 5031–5052.
- Dijk, F., Veenstra, V. L., Soer, E. C., Dings, M. P., Zhao, L., Halfwerk, J. B., Hooijer, G. K., Damhofer, H., Marzano, M., Steins, A., et al. (2020). Unsupervised class discovery in pancreatic ductal adenocarcinoma reveals cell-intrinsic mesenchymal features and high concordance between existing classification systems. *Scientific reports* **10**, 337.
- Hayashi, A., Fan, J., Chen, R., Ho, Y.-j., Makohon-Moore, A. P., Lecomte, N., Zhong, Y., Hong, J., Huang, J., Sakamoto, H., et al. (2020). A unifying paradigm for transcriptional heterogeneity and squamous features in pancreatic ductal adenocarcinoma. *Nature Cancer* **1**, 59–74.
- Ibrahim, J. G., Zhu, H., Garcia, R. I., and Guo, R. (2011). Fixed and random effects selection in mixed effects models. *Biometrics* **67**, 495–503.

Kolde, R. (2019). *pheatmap: Pretty Heatmaps*. R package version 1.0.12.

Moffitt, R. A., Marayati, R., Flate, E. L., Volmar, K. E., Loeza, S. G. H., Hoadley, K. A., Rashid, N. U., Williams, L. A., Eaton, S. C., Chung, A. H., et al. (2015). Virtual microdissection identifies distinct tumor-and stroma-specific subtypes of pancreatic ductal adenocarcinoma. *Nature genetics* **47**, 1168.

R Core Team (2021). *R: A Language and Environment for Statistical Computing*. R Foundation for Statistical Computing, Vienna, Austria.

Raphael, B. J., Hruban, R. H., Aguirre, A. J., Moffitt, R. A., Yeh, J. J., Stewart, C., Robertson, A. G., Cherniack, A. D., Gupta, M., Getz, G., et al. (2017). Integrated genomic characterization of pancreatic ductal adenocarcinoma. *Cancer cell* **32**, 185–203.

| Corr | $\pi$ | TP %<br>Fixef | FP %<br>Fixef | TP %<br>Ranef | FP %<br>Ranef | $T^{med}$ | Abs.<br>Dev.<br>(Mean) |
|------|-------|---------------|---------------|---------------|---------------|-----------|------------------------|
| 0.2  | 0.1   | 97.55         | 27.39         | 85.10         | 12.40         | 23.34     | 0.50                   |
|      | 0.3   | 91.70         | 13.32         | 61.90         | 4.46          | 22.06     | 0.54                   |
|      | 0.5   | 93.30         | 7.79          | 65.80         | 2.64          | 8.63      | 0.51                   |
|      | 0.8   | 94.10         | 1.08          | 90.00         | 0.63          | 2.58      | 0.40                   |
|      | 1.0   | 94.70         | 4.28          | 94.40         | 0.53          | 1.46      | 0.31                   |
| 0.4  | 0.1   | 86.53         | 22.79         | 74.53         | 14.33         | 14.37     | 0.56                   |
|      | 0.3   | 87.98         | 11.93         | 59.49         | 1.99          | 15.10     | 0.58                   |
|      | 0.5   | 85.70         | 4.64          | 72.70         | 1.07          | 4.71      | 0.53                   |
|      | 0.8   | 80.30         | 1.61          | 83.30         | 0.37          | 2.54      | 0.44                   |
|      | 1.0   | 80.40         | 1.98          | 82.60         | 0.21          | 1.17      | 0.39                   |
| 0.6  | 0.1   | 80.14         | 17.16         | 53.24         | 7.03          | 13.08     | 0.63                   |
|      | 0.3   | 76.39         | 10.63         | 55.26         | 3.13          | 10.31     | 0.61                   |
|      | 0.5   | 75.00         | 4.20          | 58.50         | 0.86          | 4.10      | 0.55                   |
|      | 0.8   | 76.70         | 1.28          | 64.20         | 0.61          | 2.47      | 0.45                   |
|      | 1.0   | 71.31         | 0.85          | 56.26         | 0.24          | 1.40      | 0.41                   |
| CS   | 0.1   | 93.10         | 45.41         | 92.00         | 29.90         | 28.90     | 0.49                   |
|      | 0.3   | 93.80         | 28.63         | 74.30         | 16.32         | 24.74     | 0.46                   |
|      | 0.5   | 87.90         | 19.19         | 66.60         | 11.71         | 12.78     | 0.44                   |
|      | 0.8   | 91.70         | 3.99          | 75.00         | 2.94          | 3.12      | 0.40                   |
|      | 1.0   | 95.90         | 2.04          | 86.20         | 1.38          | 1.36      | 0.30                   |

Web Table 1: Variable selection results for the Elastic Net simulations, including true positive (TP) percentages for fixed and random effects, false positive (FP) percentages for fixed and random effects, the median time in hours for the algorithm to complete ( $T^{med}$ ), and the average of the mean absolute deviation (Abs. Dev. (Mean)) between the coefficient estimates and the true  $\beta$  values across all simulation replicates. Column “Corr” describes the correlation between the covariates (equal correlation of values 0.2, 0.4, or 0.6, or correlation based on data from the case study data, labeled as ‘CS’). Column  $\pi$  represents the Elastic Net balance between ridge regression ( $\pi = 0$ ) and the MCP penalty ( $\pi = 1$ ).

| Corr | $\pi$ | Avg. $r$ | $r$ Underestimated % | $r$ Correct % | $r$ Overestimated % |
|------|-------|----------|----------------------|---------------|---------------------|
| 0.2  | 0.1   | 2.67     | 35                   | 63            | 2                   |
|      | 0.3   | 2.65     | 35                   | 65            | 0                   |
|      | 0.5   | 2.63     | 37                   | 63            | 0                   |
|      | 0.8   | 2.54     | 46                   | 54            | 0                   |
|      | 1.0   | 2.62     | 39                   | 60            | 1                   |
| 0.4  | 0.1   | 2.24     | 76                   | 24            | 0                   |
|      | 0.3   | 2.35     | 67                   | 32            | 1                   |
|      | 0.5   | 2.38     | 68                   | 28            | 4                   |
|      | 0.8   | 2.47     | 69                   | 26            | 5                   |
|      | 1.0   | 2.35     | 73                   | 24            | 3                   |
| 0.6  | 0.1   | 2.05     | 95                   | 5             | 0                   |
|      | 0.3   | 2.30     | 82                   | 12            | 5                   |
|      | 0.5   | 2.30     | 81                   | 12            | 7                   |
|      | 0.8   | 2.38     | 84                   | 8             | 8                   |
|      | 1.0   | 2.99     | 72                   | 13            | 15                  |
| CS   | 0.1   | 2.47     | 53                   | 47            | 0                   |
|      | 0.3   | 2.45     | 55                   | 45            | 0                   |
|      | 0.5   | 2.42     | 58                   | 42            | 0                   |
|      | 0.8   | 2.44     | 56                   | 44            | 0                   |
|      | 1.0   | 2.43     | 57                   | 43            | 0                   |

Web Table 2: Results of the Growth Ratio  $r$  estimation procedure for the Elastic Net  $p = 100$  logistic mixed effects simulation results, including the average estimate of  $r$  across simulations and percent of times that the estimation procedure underestimated  $r$ , gave the true  $r$ , or overestimated  $r$ . Column “Corr” describes the correlation between the covariates (equal correlation of values 0.2, 0.4, or 0.6, or correlation based on data from the case study data). Column  $\pi$  represents the Elastic Net balance between ridge regression ( $\pi = 0$ ) and the MCP penalty ( $\pi = 1$ ).

| Dataset | Platform | Sample Size | % Basal | Citation              |
|---------|----------|-------------|---------|-----------------------|
| Aguirre | RNA-seq  | 28          | 29      | Aguirre et al. (2018) |
| CPTAC   | RNA-seq  | 99          | 22      | Cao et al. (2021)     |
| Dijk    | RNA-seq  | 61          | 39      | Dijk et al. (2020)    |
| Hayashi | RNA-seq  | 75          | 53      | Hayashi et al. (2020) |
| TCGA    | RNA-seq  | 97          | 20      | Raphael et al. (2017) |

Web Table 3: Summaries of PDAC gene expression datasets. Used in case study prediction model of basal subtype.
